# Supplementary material for: Convolutional Neural Networks as 2-D systems
Source: arXiv:2303.03042 source file (2023-04-11)
Supplement: Supplementary file 1 [file appendix.tex]

\subsection{Controllability of 2-D systems}
\label{app:1}

\begin{definition}[Controllability and the controllability gramian]
    We call the 2-D system \eqref{eq:2DsysDissi} controllable if, for zero initial conditions, i.e., $x_1 [i_1,i_2] = 0$ for all $(i_1,i_2) \in \{-r\} \times \bbZ_{\geq -r}$ and $x_2[i_1,i_2] = 0$ for all $(i_1,i_2) \in \bbZ_{\geq -r} \times \{0\}$ there exist $j_1,j_2 \in \bbN$ and an input sequence $u[i_1,i_2] \in \ell_{2e}(\bbZ \times \bbZ)$ such that
    \begin{align*}
        x[j_1,j_2] = x_{\text{des}}
    \end{align*}
    furthermore, we define the Kalman matrix of \eqref{eq:2DsysDissi} as
    \begin{align*}
    \bK_{j_1,j_2}
        \begin{pmatrix}
            \bA^{j_1-1,j_2}\bB_1 + \bA^{j_1,j_2-1} \bB_2, \ldots , \bA^{0,1}\bB_1 + \bA^{1,0} \bB_2,\bB_1 + \bB_2
        \end{pmatrix},
    \end{align*}
    where the matrices $\bA^{i_1,i_2}$ and $\bB_1,\bB_2$ are defined by
    \begin{align*}
        \bB_1 = \begin{pmatrix}
            \bB_1\\
            0
        \end{pmatrix},
        \bB_2 = \begin{pmatrix}
            0\\ \bB_2
        \end{pmatrix},
        \bA^{1,0} = \begin{pmatrix}
            \bA_{11} & \bA_{12}\\
            0 & 0
        \end{pmatrix},
        \bA^{0,1} = \begin{pmatrix}
            0 & 0\\
            \bA_{12} & \bA_{22}
        \end{pmatrix},
        \bA^{i_1,i_2} = \bA^{1,0} \bA^{i_1-1,i_2} + \bA^{0,1} \bA^{i_1,i_2-1}
    \end{align*}
\end{definition}

The controllable subspace can be defined accordingly as $\calV_{\mathrm{cont}} = \bigcup_{j_1,j_2=0}^\infty \mathrm{im} \bP_{j_1,j_2}$. It can be shown \cite{}, that the 2-D system \eqref{eq:2DsysDissi} is controllable if $\dim \calV_{\mathrm{cont}} = n_1 + n_2$
